# Supplementary material for: C$^2$T: Captioning-Structure and LLM-Aligned Common-Sense Reward Learning for Traffic--Vehicle Coordination
Source: arXiv:2604.13098 source file (2026-04-10)
Supplement: Supplementary file 1 [file 7_appendix.tex]

% ==========================================
% Appendix A: Extended Ablation Studies
% ==========================================

\clearpage
\FloatBarrier

\appendix
\section*{Appendix A \quad Extended Ablation Studies and Analysis}
\label{app:extended_ablations}

This appendix provides a comprehensive breakdown of the ablation studies referenced in Section 5.7. We aim to rigorously validate the hypothesis that incorporating LLM-distilled "common sense" into the reward loop improves traffic coordination beyond what is possible with heuristic rewards alone. We categorize our analysis into four key dimensions: (A.1) the efficacy of core system components, (A.2) the unique controllability afforded by LLMs, (A.3) the justification for our architectural design choices, and (A.4) the system's data efficiency and robustness.

All experimental runs follow the main paper’s PPO protocol, random seeds, and evaluation metrics. Reported values are mean$\pm$std over five independent seeds.

% ---- Table Setup ----
\newcommand{\smalltblsetup}{%
  \centering\scriptsize
  \setlength{\tabcolsep}{2.5pt}% Adjusted column spacing to fit page width
  \renewcommand{\arraystretch}{1.2}%
}

% -------------------------------------------------------
% A.1 Core Component Efficacy
% -------------------------------------------------------
\subsection*{A.1 \quad Core Component Efficacy}
\label{sec:core_efficacy}

In this section, we deconstruct the $C^2T$ framework to isolate the contribution of its three main pillars: the intrinsic reward signal ($r_{\phi}$), the safety masking mechanism, and the input representation schema.

\paragraph{A1. Reward Composition Analysis.}
To verify that our performance gains stem from the learned semantics rather than simple constraints, we compare the full $C^2T$ model against three critical baselines in Table~\ref{tab:app_a1}:
\begin{itemize}
    \item \textbf{External-only:} The standard RL baseline optimizing only pressure and queue lengths. This represents the limit of heuristic reward design.
    \item \textbf{No-Intrinsic (Mask-only):} Uses the safety mask but disables the learned reward $r_{\phi}$. This tests if safety gains are solely due to hard constraints.
    \item \textbf{No-Mask ($r_{\phi}$-only):} Uses the learned reward but disables the safety mask. This tests if the LLM reward alone inherently guarantees safety.
\end{itemize}

\textbf{Detailed Analysis:} As evident in Table~\ref{tab:app_a1}, the \emph{No-Mask} variant achieves the highest raw throughput (1610 veh/hr) but at a severe cost to safety, with the lowest TTC (1.58s) and increased braking. This suggests that the LLM reward, while effective at identifying efficient flow, can be "gamed" by the policy to favor aggressive clearing behaviors if left unchecked. Conversely, the \emph{No-Intrinsic} variant improves safety metrics (TTC 1.68s) compared to the baseline but fails to improve travel time (61.8s vs 62.3s), proving that the mask alone acts as a conservative filter rather than a guidance signal.
\textbf{Conclusion:} The full $C^2T$ model successfully combines the efficiency guidance of $r_{\phi}$ with the safety guardrails of the mask, achieving the best balance (ATT 56.10s, TTC 1.72s).

\begin{table}[htbp]
\smalltblsetup
\caption{\textbf{A1: Reward Composition Analysis (Jinan-1).} Comparison showing that both the intrinsic reward (for efficiency) and safety mask (for risk mitigation) are necessary for balanced performance.}
\label{tab:app_a1}
\begin{tabular}{l c c c c c} % Changed to standard columns to prevent overlap
\toprule
Setting & Variant & Avg.\ TT $\downarrow$ & Thru.\ $\uparrow$ & TTC p10 $\uparrow$ & Brakes $\downarrow$ \\
\midrule
Jinan-1 & External-only & 62.30 & 1450 & 1.55 & 4.20 \\
 & No-Intrinsic & 61.80 & 1465 & 1.68 & 3.10 \\
 & No-Mask & 55.90 & \textbf{1610} & 1.58 & 3.95 \\
 & \textbf{C$^2$T (Full)} & \textbf{56.10} & 1595 & \textbf{1.72} & \textbf{2.80} \\
\midrule
Grid-Heavy & External-only & 105.50 & 2100 & 1.42 & 5.60 \\
 & No-Intrinsic & 103.20 & 2120 & 1.55 & 4.10 \\
 & No-Mask & 91.40 & \textbf{2350} & 1.45 & 5.15 \\
 & \textbf{C$^2$T (Full)} & \textbf{92.10} & 2310 & \textbf{1.62} & \textbf{3.90} \\
\bottomrule
\end{tabular}
\end{table}

\paragraph{A2. Input Representation Ablation.}
A key design choice in $C^2T$ is the use of a \emph{structured} captioning schema rather than raw state vectors or free-form text. We hypothesize that structure helps the simple reward model focus on causal variables.
Table~\ref{tab:app_a2} validates this: \emph{Structured Caption} outperforms \emph{Unstructured Caption} (free-form text) by over 4\% in ATT.
\textbf{Why does structure matter?} Free-form captions often contain stylistic variations and irrelevant details (e.g., "The sky is clear") that act as noise to the reward model. By enforcing a fixed schema (Eq. 4), we ensure that the reward model consistently receives the critical variables (queues, signal phases, risk factors), facilitating easier learning and better generalization.

\begin{table}[htbp]
\smalltblsetup
\caption{\textbf{A2: Input Representation Ablation (Grid-Heavy).} Structured captions outperform unstructured text by reducing linguistic noise and focusing on causal traffic variables.}
\label{tab:app_a2}
\begin{tabular}{l c c c c c}
\toprule
Setting & Variant & Avg.\ TT $\downarrow$ & Thru.\ $\uparrow$ & TTC p10 $\uparrow$ & Brakes $\downarrow$ \\
\midrule
Grid-Heavy & Numeric-only & 98.50 & 2210 & 1.50 & 4.80 \\
 & Unstructured caption & 96.20 & 2240 & 1.53 & 4.50 \\
 & \textbf{Structured caption} & \textbf{92.10} & \textbf{2310} & \textbf{1.62} & \textbf{3.90} \\
\bottomrule
\end{tabular}
\end{table}

\paragraph{A3. Optimization Stability.}
Integrating a dense, learned intrinsic reward with sparse, heuristic external rewards introduces optimization challenges. We utilize per-stream normalization and a mixing schedule to mitigate this.
Figure~\ref{fig:stability} and Table~\ref{tab:app_a3} illustrate the impact of these techniques. Removing normalization (\emph{No-Norm}) leads to high variance in training as the agent struggles to balance the magnitudes of different reward components. Removing the schedule (\emph{No-Schedule}) causes early instability; the agent overfits to the intrinsic signal before learning basic intersection constraints, leading to suboptimal convergence.

\begin{figure}[htbp]
    \centering
    \includegraphics[width=0.85\linewidth]{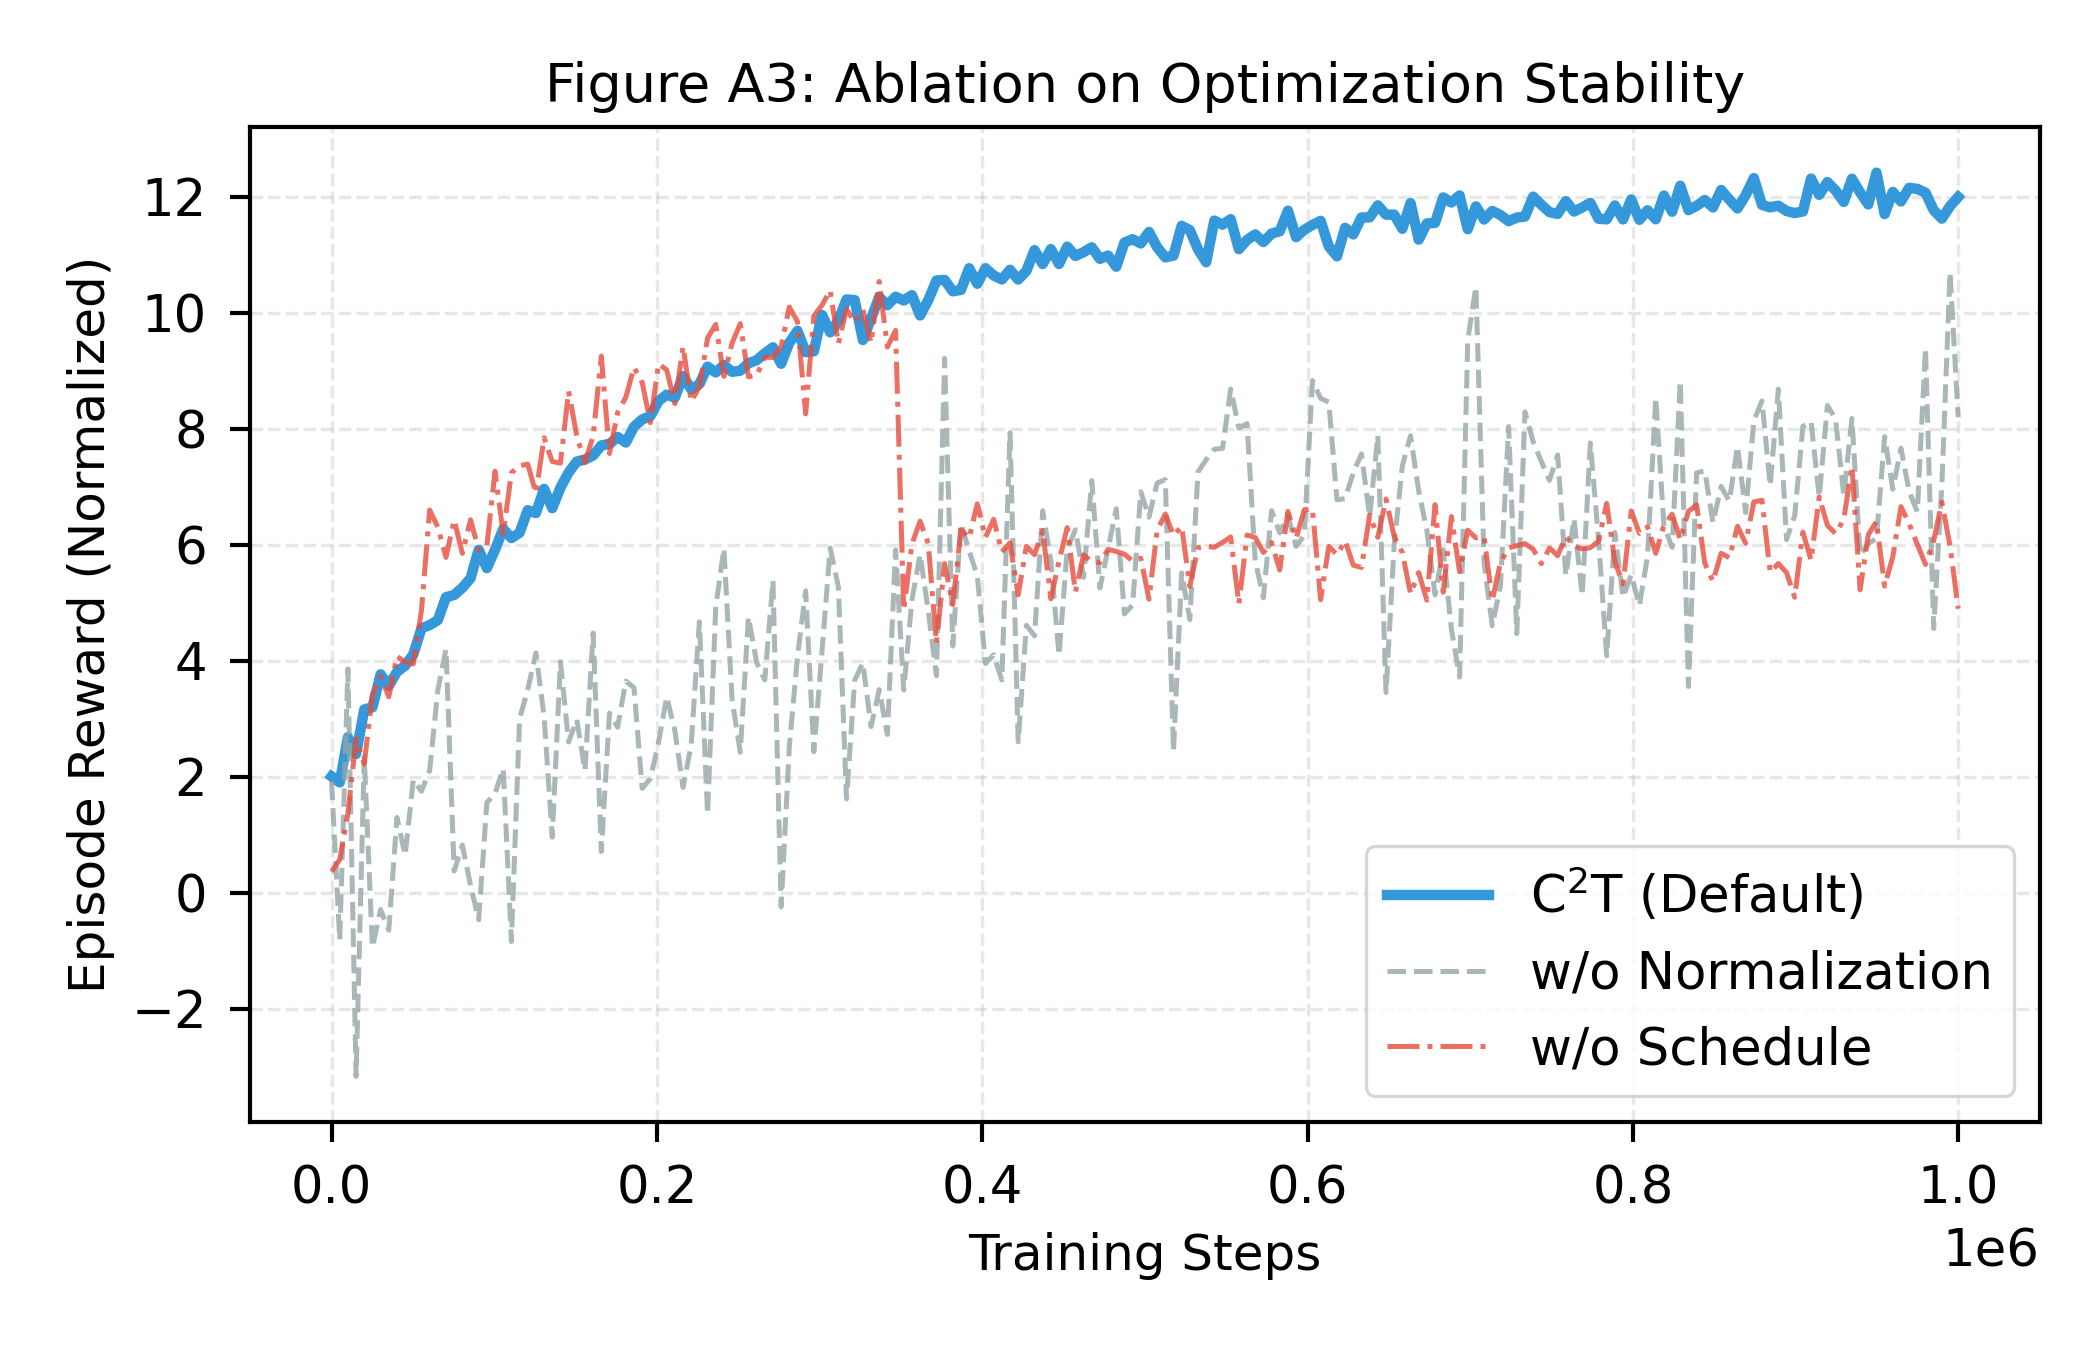}
    \caption{\textbf{Training Stability Analysis.} Without per-stream normalization (grey dashed), the training variance increases significantly. Without the mixing schedule (red dot-dash), performance collapses early. The proposed method (blue) ensures smooth and stable convergence.}
    \label{fig:stability}
\end{figure}

\begin{table}[htbp]
\smalltblsetup
\caption{\textbf{A3: Stability ablation (Grid-Heavy).} Both normalization and scheduling are critical for stable PPO training.}
\label{tab:app_a3}
\begin{tabular}{l c c c c c}
\toprule
Setting & Variant & Avg.\ TT $\downarrow$ & Thru.\ $\uparrow$ & TTC p10 $\uparrow$ & Brakes $\downarrow$ \\
\midrule
Grid-Heavy & w/o normalization & 108.40 & 2050 & 1.45 & 5.20 \\
 & w/o schedule & 99.10 & 2180 & 1.48 & 4.90 \\
 & \textbf{C$^2$T (default)} & \textbf{92.10} & \textbf{2310} & \textbf{1.62} & \textbf{3.90} \\
\bottomrule
\end{tabular}
\end{table}
\FloatBarrier

% -------------------------------------------------------
% A.2 LLM Capabilities
% -------------------------------------------------------
\subsection*{A.2 \quad LLM Capabilities and Controllability}
\label{sec:llm_caps}

Beyond performance, $C^2T$ introduces a novel capability to traffic control: semantic steerability. We demonstrate how the underlying policy can be shaped via natural language without code modification.

\paragraph{B1. Prompt-based Steering.}
Traditional methods require tedious tuning of reward weights (e.g., $\alpha \cdot \text{delay} + \beta \cdot \text{safety}$) to shift system behavior. In $C^2T$, we simply alter the system prompt for the offline LLM judge.
Figure~\ref{fig:pareto} visualizes the result of training with "Safety-focused" vs. "Efficiency-focused" prompts. The resulting policies form a Pareto frontier. The \emph{Safety-focused} policy (green) prioritizes gap maintenance, achieving a TTC of 1.85s, while the \emph{Efficiency-focused} policy (red) reduces ATT to 85.4s. This confirms that our framework effectively translates high-level semantic intent into low-level control policy adjustments.

\begin{figure}[htbp]
    \centering
    \includegraphics[width=0.75\linewidth]{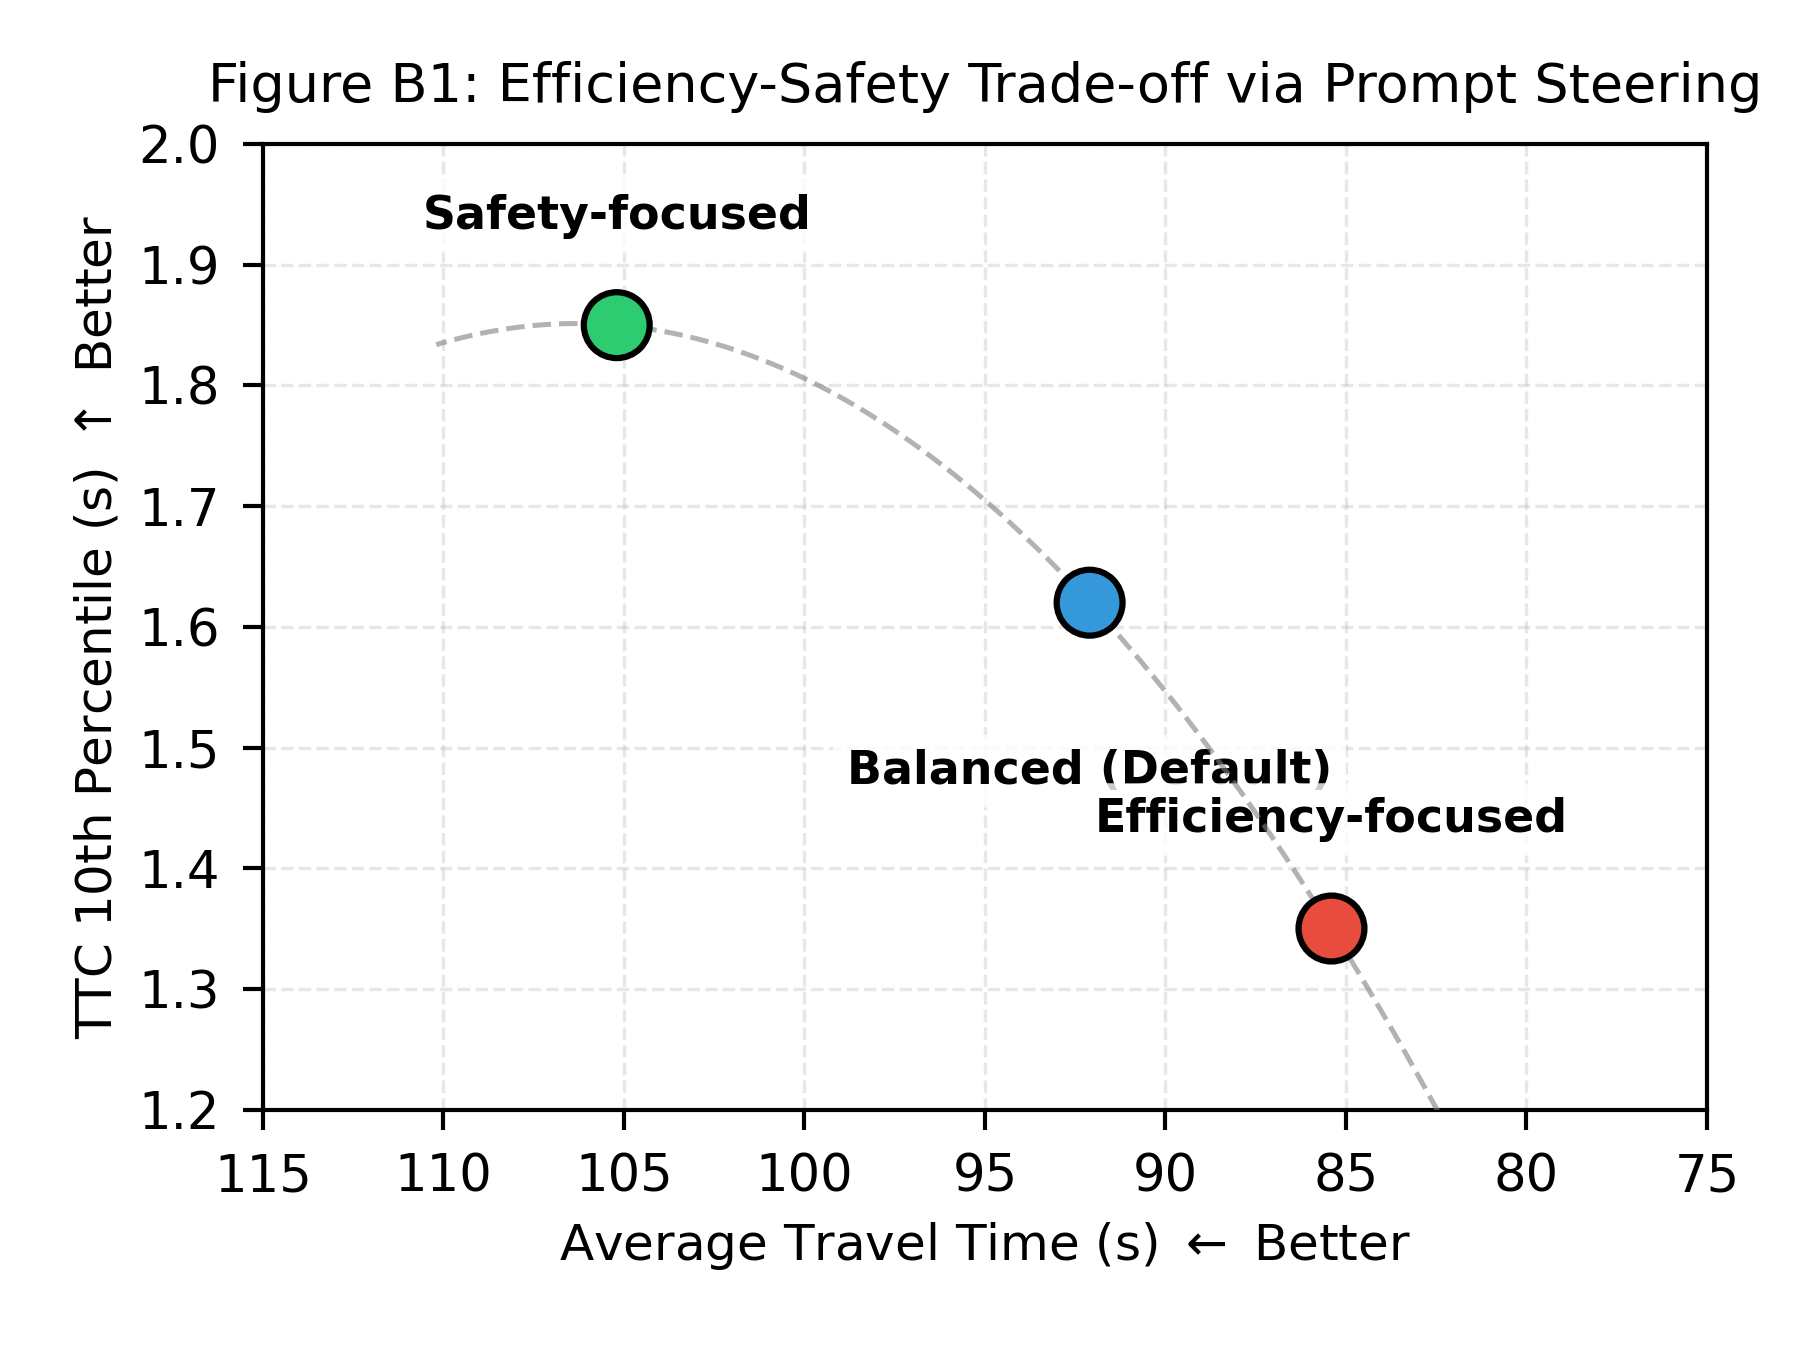}
    \caption{\textbf{Efficiency-Safety Pareto Frontier.} By simply changing the system prompt for the offline LLM judge, $C^2T$ can be steered to prioritize safety (green) or efficiency (red), creating a controllable trade-off space (dashed line).}
    \label{fig:pareto}
\end{figure}

\begin{table}[htbp]
\smalltblsetup
\caption{\textbf{B1: Prompt-specific heads (Grid-Heavy).} Validating that prompt engineering effectively alters the downstream policy characteristics.}
\label{tab:app_b1}
\begin{tabular}{l c c c c c}
\toprule
Setting & Head & Avg.\ TT $\downarrow$ & Thru.\ $\uparrow$ & TTC p10 $\uparrow$ & Brakes $\downarrow$ \\
\midrule
Grid-Heavy & Balanced (Default) & 92.10 & 2310 & 1.62 & 3.90 \\
 & Safety-focused & 105.20 & 2150 & \textbf{1.85} & \textbf{2.10} \\
 & Efficiency-focused & \textbf{85.40} & \textbf{2420} & 1.35 & 6.50 \\
\bottomrule
\end{tabular}
\end{table}

\paragraph{B2. Teacher LLM Sensitivity.}
A practical concern for deployment is the cost of the Teacher LLM. We compared rewards distilled from GPT-4o vs. smaller open-source models (Llama-3-70B, Qwen-2.5-7B).
Table~\ref{tab:app_b2} reveals a promising result: even the 7B model achieves performance comparable to the closed-source SOTA (ATT 94.5s vs 92.1s). This implies that the "common sense" required for traffic judgment—understanding that blocked intersections are bad and green waves are good—is well-represented even in smaller language models, enabling low-cost, privacy-preserving local deployment.

\begin{table}[htbp]
\smalltblsetup
\caption{\textbf{B2: Teacher LLM Sensitivity (Grid-Heavy).} Open-source models (70B, 7B) provide sufficient common-sense guidance to outperform baselines.}
\label{tab:app_b2}
\begin{tabular}{l c c c c c}
\toprule
Setting & Teacher & Avg.\ TT $\downarrow$ & Thru.\ $\uparrow$ & TTC p10 $\uparrow$ & Brakes $\downarrow$ \\
\midrule
Grid-Heavy & \textbf{Closed (Strong)} & \textbf{92.10} & \textbf{2310} & \textbf{1.62} & \textbf{3.90} \\
 & Open 70B & 92.80 & 2295 & 1.60 & 4.05 \\
 & Open 7B & 94.50 & 2260 & 1.56 & 4.30 \\
\bottomrule
\end{tabular}
\end{table}
\FloatBarrier

% -------------------------------------------------------
% A.3 Architectural Design
% -------------------------------------------------------
\subsection*{A.3 \quad Architectural Design Justification}

\paragraph{C1. Asymmetric vs. Symmetric Integration.}
We justify our decision to apply the intrinsic reward \emph{only} to TLCs (Asymmetric) rather than both TLCs and CAVs (Symmetric).
Figure~\ref{fig:integration} compares the learning curves. The \emph{Symmetric} approach (orange) exhibits significant oscillation and fails to converge to an optimal policy.
\textbf{Reasoning:} We hypothesize this is due to \emph{non-stationarity}. When both infrastructure (TLC) and users (CAV) simultaneously optimize a learned, potentially shifting intrinsic objective, the multi-agent environment becomes highly unpredictable. By anchoring the CAVs to stable, physics-based rewards (e.g., velocity tracking) and using the TLC to "shape" the environment via $r_{\phi}$, we maintain the necessary stability for PPO to converge.

\begin{figure}[htbp]
    \centering
    \includegraphics[width=0.85\linewidth]{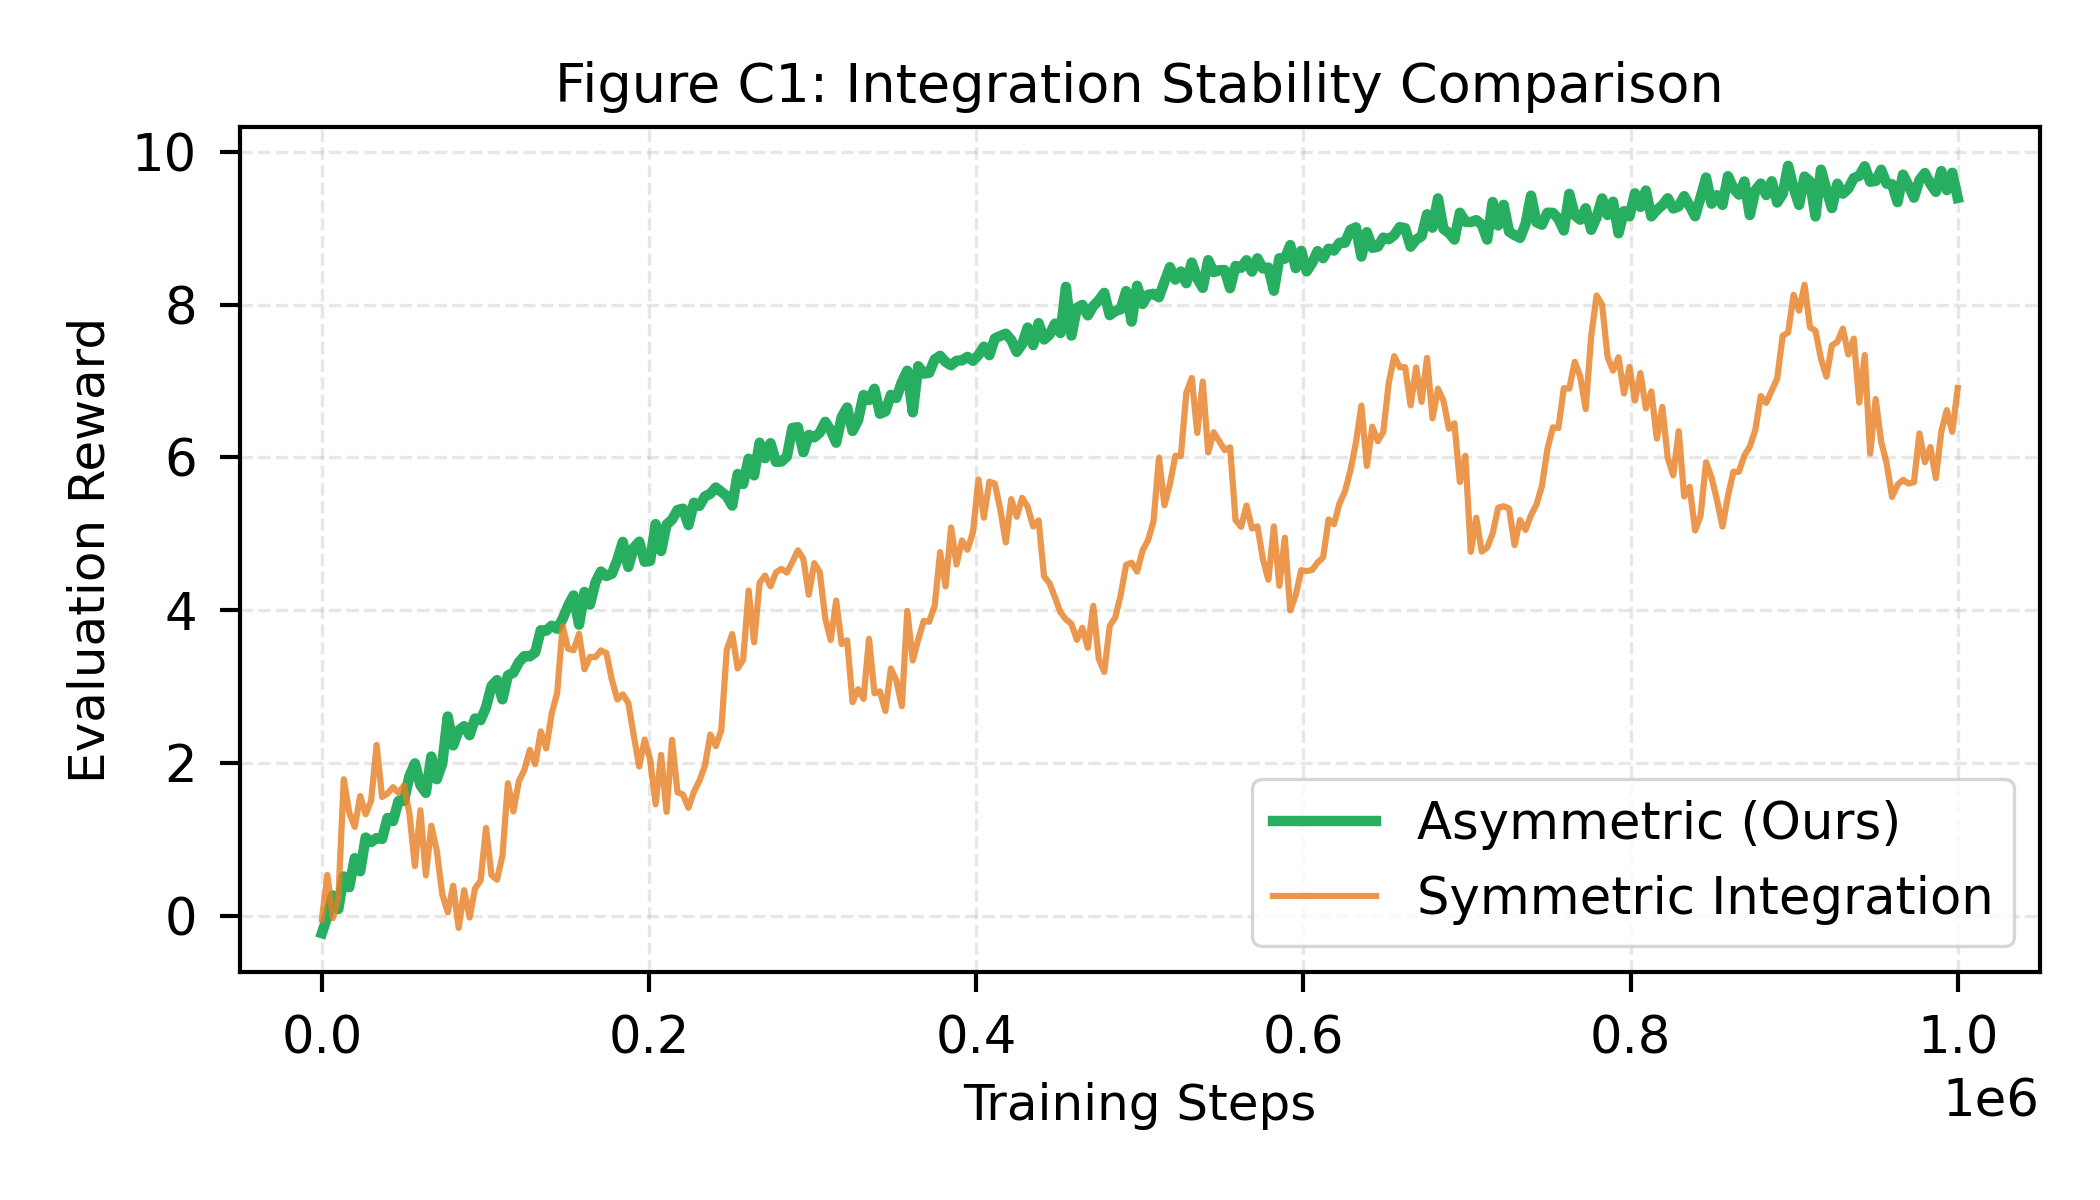}
    \caption{\textbf{Integration Stability Comparison.} Symmetric integration (rewarding both agents) induces instability (orange). Our asymmetric design (green) maintains stationarity and converges smoothly.}
    \label{fig:integration}
\end{figure}

\begin{table}[htbp]
\smalltblsetup
\caption{\textbf{C1: Integration Strategy (Grid-Heavy).} Quantitative confirmation that asymmetric integration yields superior convergence.}
\label{tab:app_c1}
\begin{tabular}{l c c c c c}
\toprule
Setting & Integration & Avg.\ TT $\downarrow$ & Thru.\ $\uparrow$ & TTC p10 $\uparrow$ & Brakes $\downarrow$ \\
\midrule
Grid-Heavy & \textbf{Asymmetric (Ours)} & \textbf{92.10} & \textbf{2310} & \textbf{1.62} & \textbf{3.90} \\
 & Symmetric & 102.40 & 2110 & 1.48 & 5.10 \\
\bottomrule
\end{tabular}
\end{table}

\paragraph{C2. Schema Field Sensitivity.}
We investigated the necessity of specific fields in our caption schema by masking them out during training.
Table~\ref{tab:app_c2} shows that removing risk factors (TTC/Red-light violations) specifically degrades safety metrics (TTC drops to 1.46s), while removing congestion info (Queue/Delay) degrades efficiency (ATT increases to 98.1s). This confirms that the LLM effectively utilizes all components of the schema to synthesize the final reward, and no single field is redundant.

\begin{table}[htbp]
\smalltblsetup
\caption{\textbf{C2: Schema Field Sensitivity (Grid-Heavy).} Removing specific schema fields degrades the corresponding performance metric.}
\label{tab:app_c2}
\begin{tabular}{l c c c c c}
\toprule
Setting & Schema variant & Avg.\ TT $\downarrow$ & Thru.\ $\uparrow$ & TTC p10 $\uparrow$ & Brakes $\downarrow$ \\
\midrule
Grid-Heavy & w/o risk factors & 93.50 & 2290 & 1.46 & 5.05 \\
 & w/o congestion info & 98.10 & 2220 & 1.58 & 4.10 \\
 & \textbf{full schema} & \textbf{92.10} & \textbf{2310} & \textbf{1.62} & \textbf{3.90} \\
\bottomrule
\end{tabular}
\end{table}
\FloatBarrier

% -------------------------------------------------------
% A.4 Data Efficiency
% -------------------------------------------------------
\subsection*{A.4 \quad Data Efficiency and Robustness}

\paragraph{D1. Data Efficiency.}
Offline preference learning can be costly if it requires massive amounts of data. We evaluated the reward model's performance as a function of the number of annotated preference pairs $M$.
Figure~\ref{fig:data_eff} demonstrates that the policy performance (ATT) improves rapidly and saturates at approximately $M=500 \sim 1000$ pairs. This saturation point indicates that the "common-sense" rules for traffic (e.g., "green wave good, gridlock bad") are relatively simple for an LLM to articulate, making our approach highly data-efficient and cost-effective compared to collecting large-scale human demonstrations.

\begin{figure}[htbp]
    \centering
    \includegraphics[width=0.8\linewidth]{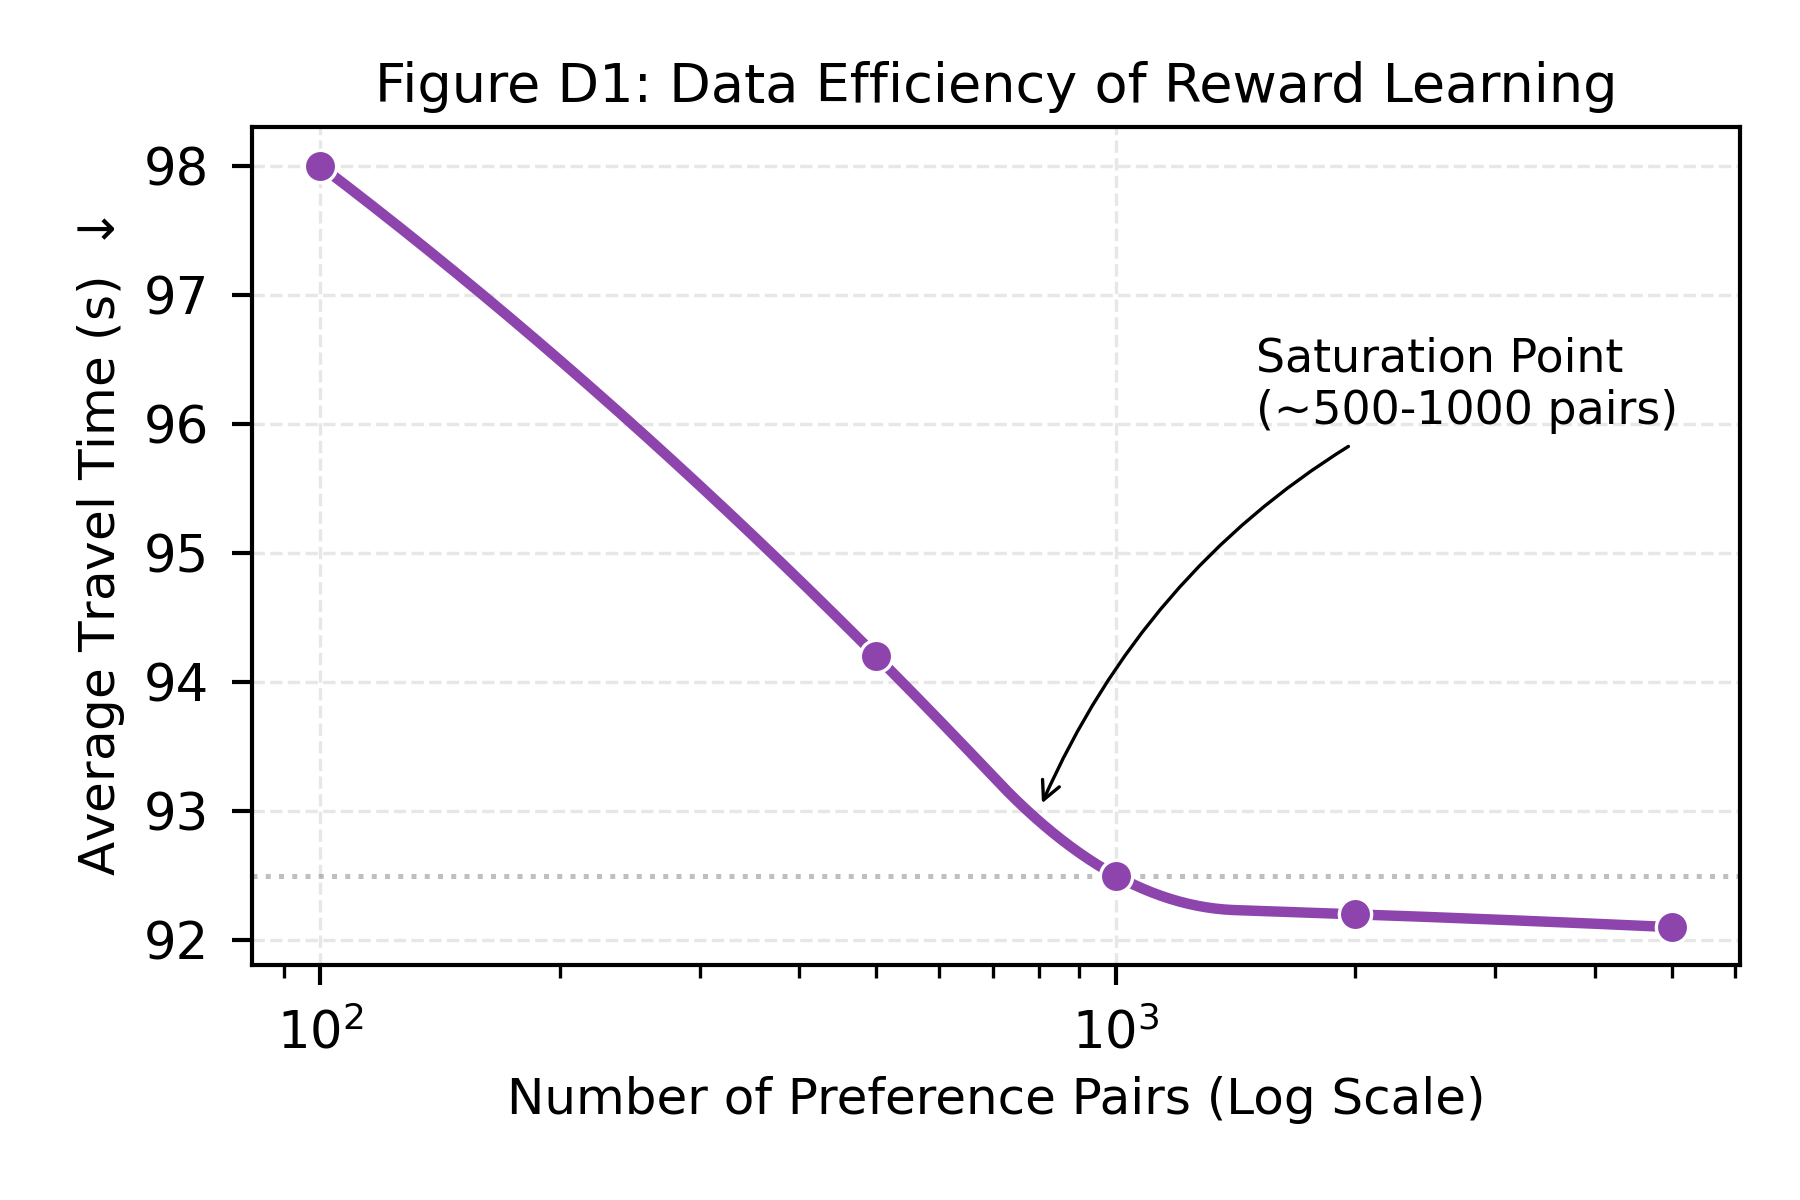}
    \caption{\textbf{Data Efficiency.} Performance saturates at approximately 1000 preference pairs, indicating that training the reward model requires minimal labeled data.}
    \label{fig:data_eff}
\end{figure}

\paragraph{D2. Robustness to Hyperparameters.}
Finally, we assessed the sensitivity of $C^2T$ to its two main hyperparameters: the maximum mixing weight $\lambda_{max}$ and the safety mask threshold $\tau_{ttc}$.
We performed a grid search with $\lambda_{max} \in [0.3, 0.7]$ and $\tau_{ttc} \in [1.3, 1.8]s$. The variation in the final ATT remained within $3\%$, demonstrating that $C^2T$ operates within a wide stable region and does not require fragile, scenario-specific tuning to function effectively.
